# Supplementary material for: Improving Weakly Supervised Visual Grounding by Contrastive Knowledge Distillation
Source: arXiv:2007.01951 source file (2021-04-25)
Supplement: Supplementary file 1 [file 04853-supp.tex]

In this section, we provide further ablation analysis of our knowledge distillation scheme and plot additional visualization of region-phrase matching.

%%%%%%%%%%%%%%%%%%%%%%%%%%%%%%%%%%%%%%%%%%%%%%%%%%%%%%%%%%%%%%%%%%%%%%%%%%
\textbf{The Effectiveness of Distillation on Phrase Localization}
We further compare the results between our model using only contrastive loss (NCE) and our full model (NCE+Distill) by breaking down the results presented in our ablation study (Table 4).

\subsection{Per-category localization accuracy}

\begin{table*}[th!]
  \small
  \centering
  \resizebox{0.9\columnwidth}{!}{
  \begin{tabular}{lcccccccc}
    \toprule
   \parbox{3cm}{Method} &
   people & clothing & body parts & animals & vehicles & instruments & scene & other\\ \midrule
%   GroundeR & 44.32 & 9.02 & 0.96 & 46.91 & 46.00 & 19.14 & 28.23 & 16.98 \\
%   UTG (YOLOv2 CC) & 58.37 & 14.87 & 2.29 & 68.91 & 55.00 & 22.22 & 24.87 & 20.77 \\
%   KAC (VGG16 CC) & 58.42 & 7.63 & 2.97 & 77.80 & 69.00 & 20.37 & 43.53 & 17.05 \\
%   WPT (IRV2 CC+IRV2 OI+WRN18 PL) & 66.27 & 37.55 & 20.65 & 84.75 & 80.00 & 47.53 & 38.91 & 34.41 \\
%   \midrule

   NCE & 64.12 & 37.57 & 9.75 & 77.49 &  72.70 & 54.90 & 34.05 & 34.81 \\
   NCE+Distill & 66.20 & 40.74 & 15.77 & 76.89 & 75.21 & 60.13 & 37.15 & 35.63 \\
%   NCE & 60.09 & 54.52 & 22.20 & 60.76 &  57.38 & 23.53 & 51.58 & 38.40 \\
%   NCE+Distillation (IRV2 OI) & 61.48 & 56.44 & 24.69 & 68.73 & 61.00 & 21.57 & 55.32 & 38.86 \\
    \bottomrule
  \end{tabular}
}\vspace{-0.5em}
\caption{Per-category phrase localization accuracy(\%) of the NCE model and NCE+Distill model on the Flickr30K Entities dataset. Both models use Res101 CC as backbone. The NCE+Distillation model uses IRV2 OI as Detector$_{K}$.} \label{tab:flickr30k-per-category}\vspace{-1.5em}
\end{table*}

Table\ \ref{tab:flickr30k-per-category} shows the per-category phrase localization accuracy on Flickr30K Entities dataset. Comparing with the NCE model, the NCE+Distill model has the largest relative improvement on following categories: body parts ($+62\%$), instruments ($+9.5\%$), scene ($+9\%$), and clothing ($+8\%$). These categories mainly contain phrases that are covered by the Open Images object classes.

\subsection{Per-phrase localization accuracy on phrases correspond to detector classes}

Fig.\ \ref{fig:phrase-accuracy} shows the accuracy of the NCE only and the NCE+Distill model on the most frequent phrase categories in Flickr30K Entities~\cite{plummer2015flickr30k} that are also presented in Open Images~\cite{krasin2017openimages}. The goal of this experiment is to verify if our distillation scheme can help to improve the accuracy of phrase categories by leveraging external knowledge from the object detector. Across all 14 categories, our full model performs on par with NCE for mouth and jeans, and outperforms NCE for 12 categories including people and clothing. We note the category of ``mouth'' has  zero accuracy for both models. This is indeed bounded by the object proposals --- only 10\% of the ``mouth'' was covered by the proposals, leading to unsatisfactory performance of both models. 

\begin{figure*}[t]
\centering
\includegraphics[width=0.8\textwidth]{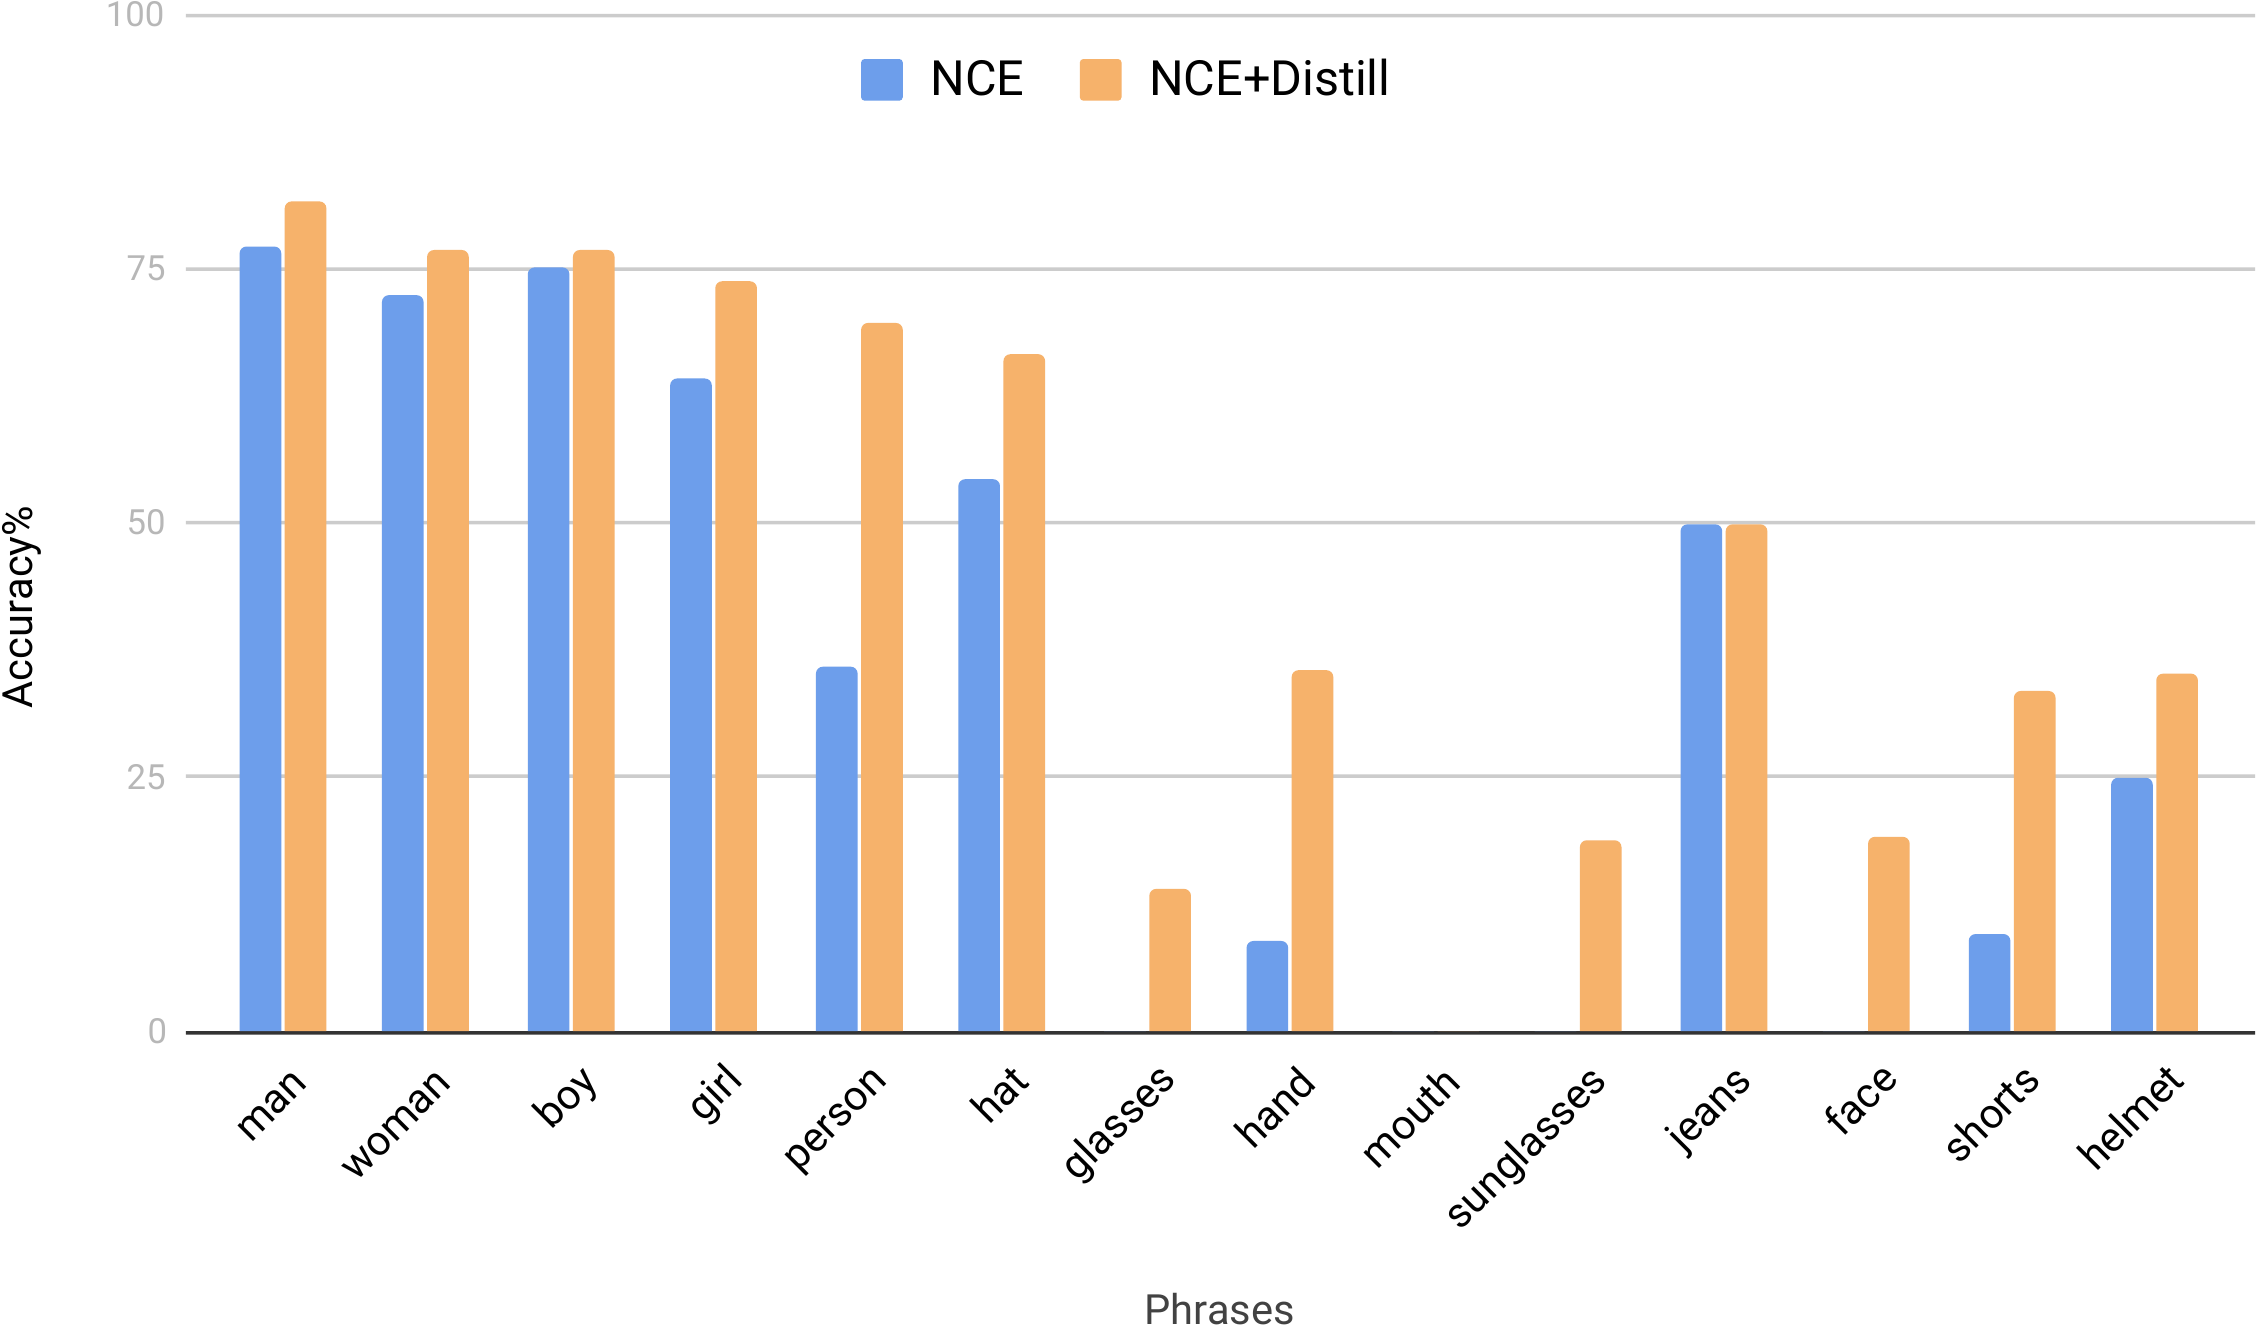}
 \caption{Phrase grounding accuracy(\%) for frequent phrases on Flickr30K Entities that are also presented in Open Images detector. We compare the results of two variants of our model (NCE vs.\ NCE+Distill). Our full model (NCE+Distill) helps to improve those phrase categories that lie in Open Images.}
\label{fig:phrase-accuracy}
\end{figure*}

%%%%%%%%%%%%%%%%%%%%%%%%%%%%%%%%%%%%%%%%%%%%%%%%%%%%%%%%%%%%%%%%%%%%%%%%%%
\section{Visualization of Region-Phrase Matching}
Moving forward, we provide additional visualization of our learned region-phrase matching function, as shown in Fig.\ \ref{fig:grounding-flickr} (samples from Flickr30K Entities~\cite{plummer2015flickr30k}) and  Fig.\ \ref{fig:grounding-referit} (samples from ReferItGame~\cite{kazemzadeh2014referitgame}). On both datasets, our learned matching function can identify meaningful regions associated with the phrases, as shown in Figures~\ref{fig:grounding-flickr} and~\ref{fig:grounding-referit}.

\begin{figure*}[th!]
\centering
\includegraphics[width=1.0\textwidth]{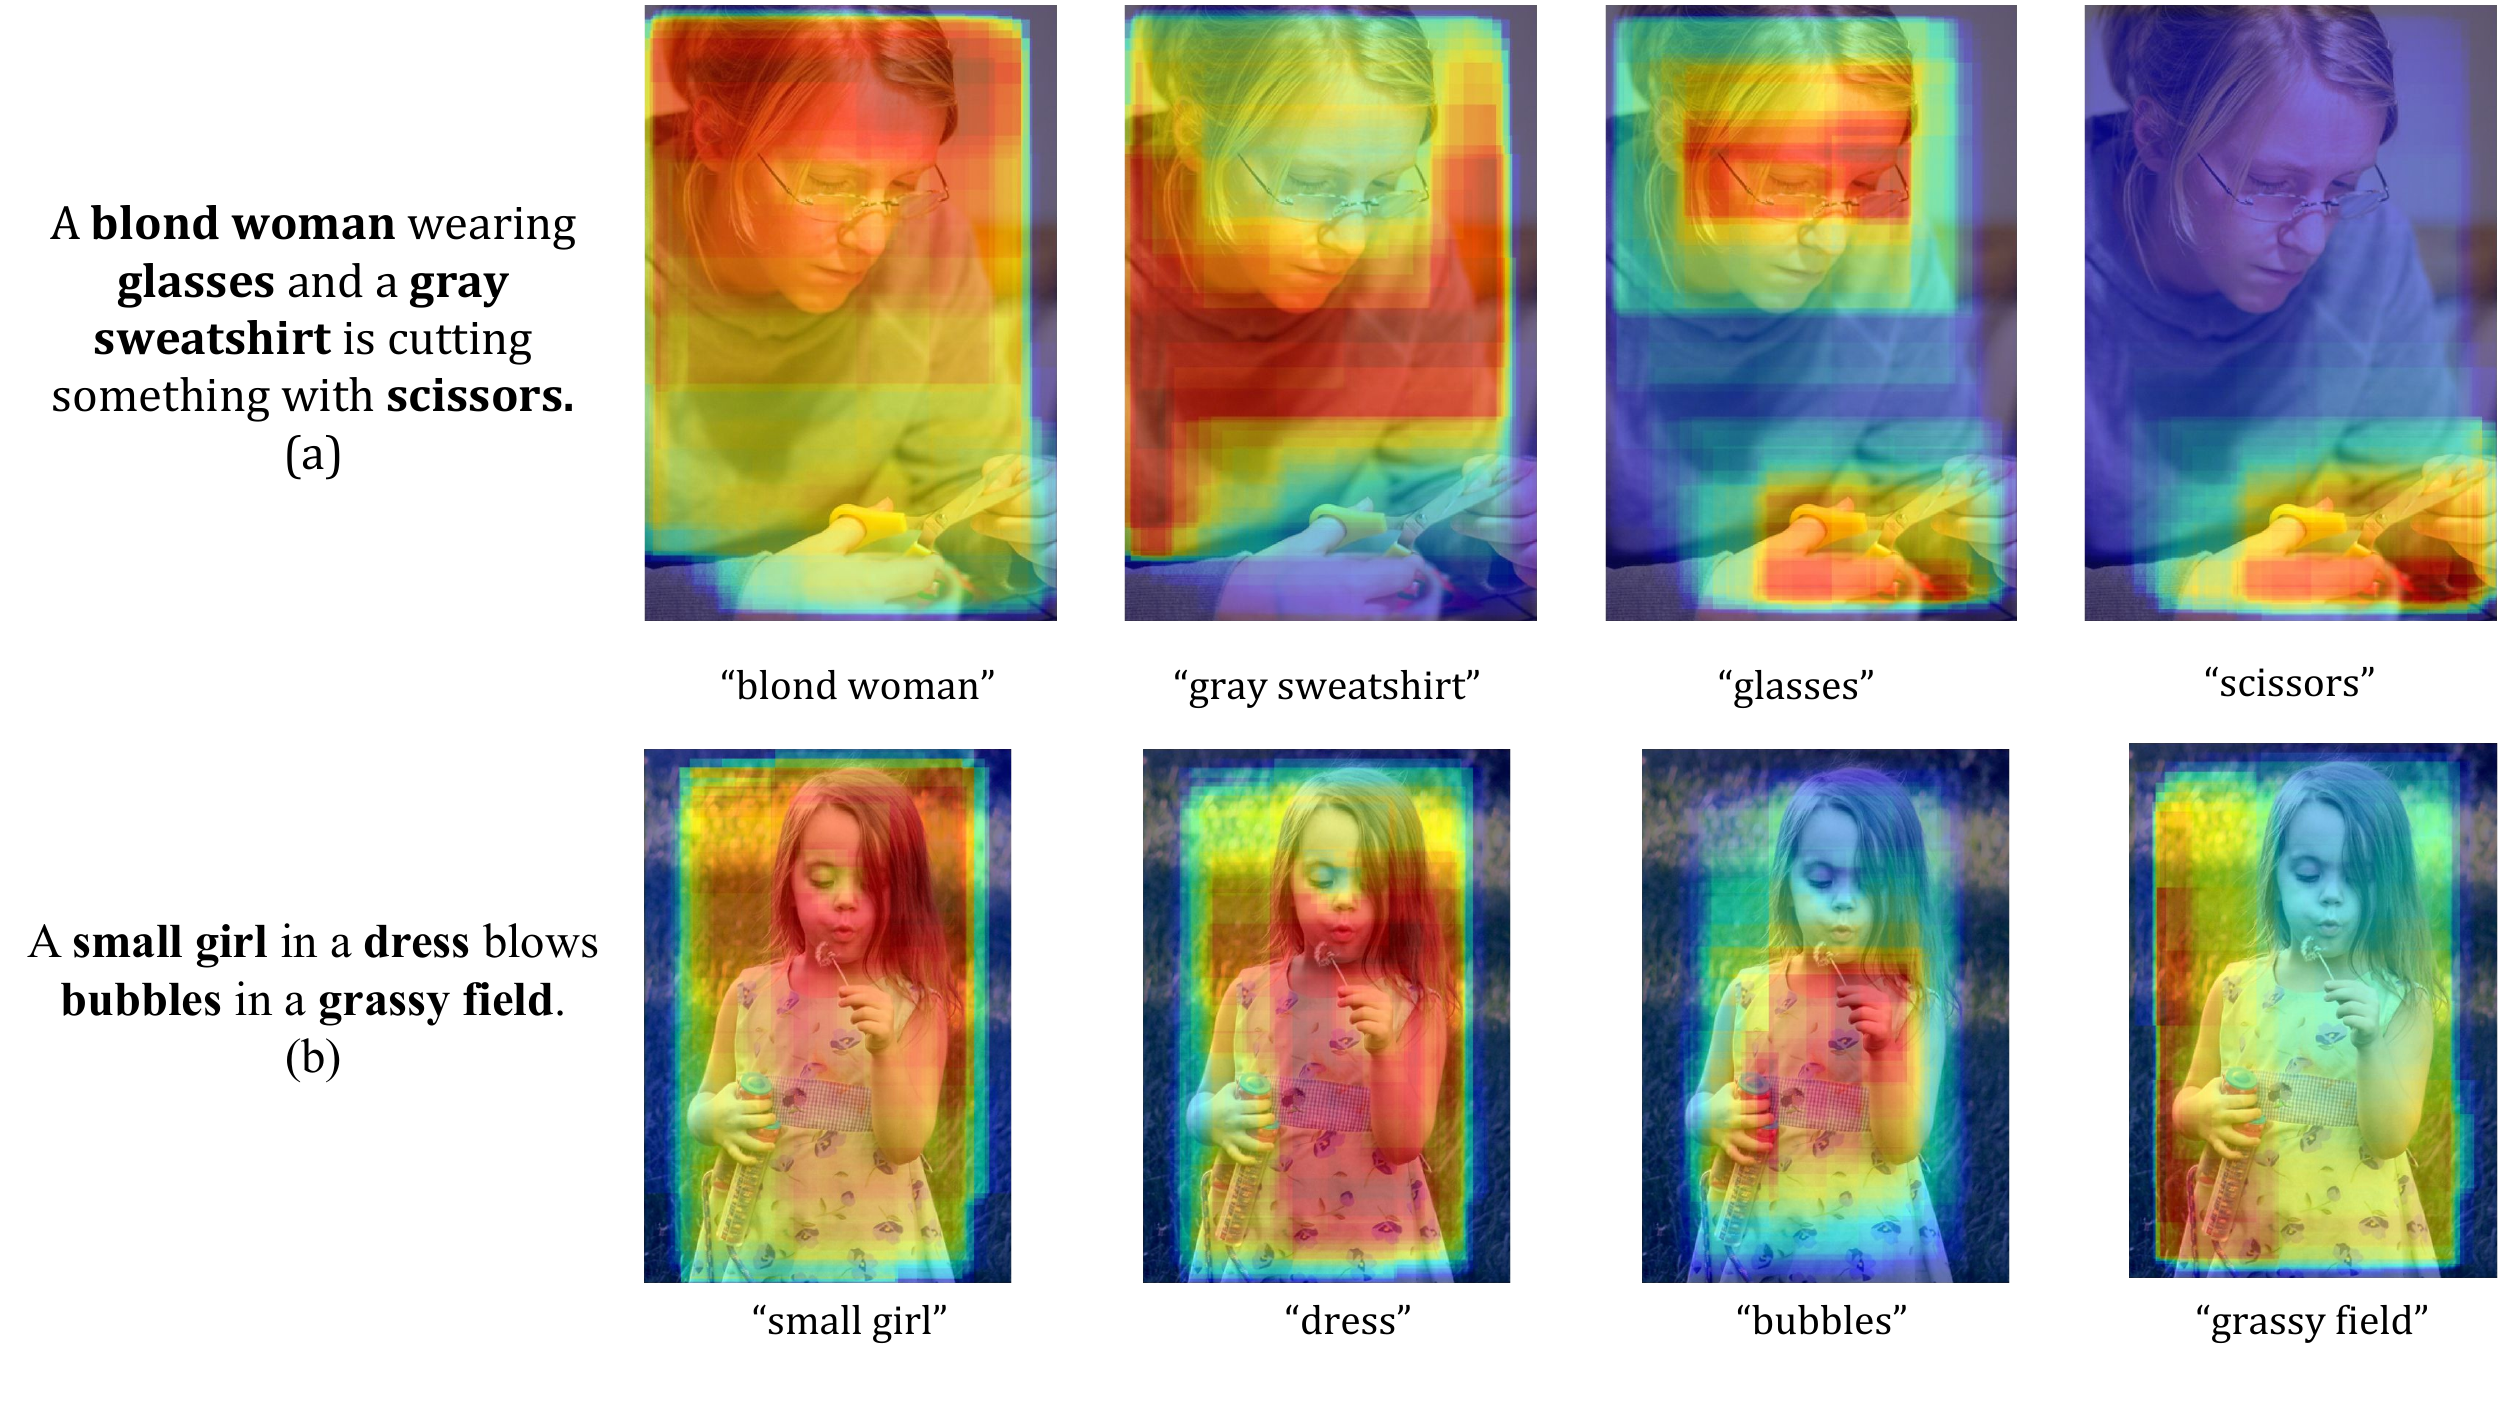}
\includegraphics[width=1.0\textwidth]{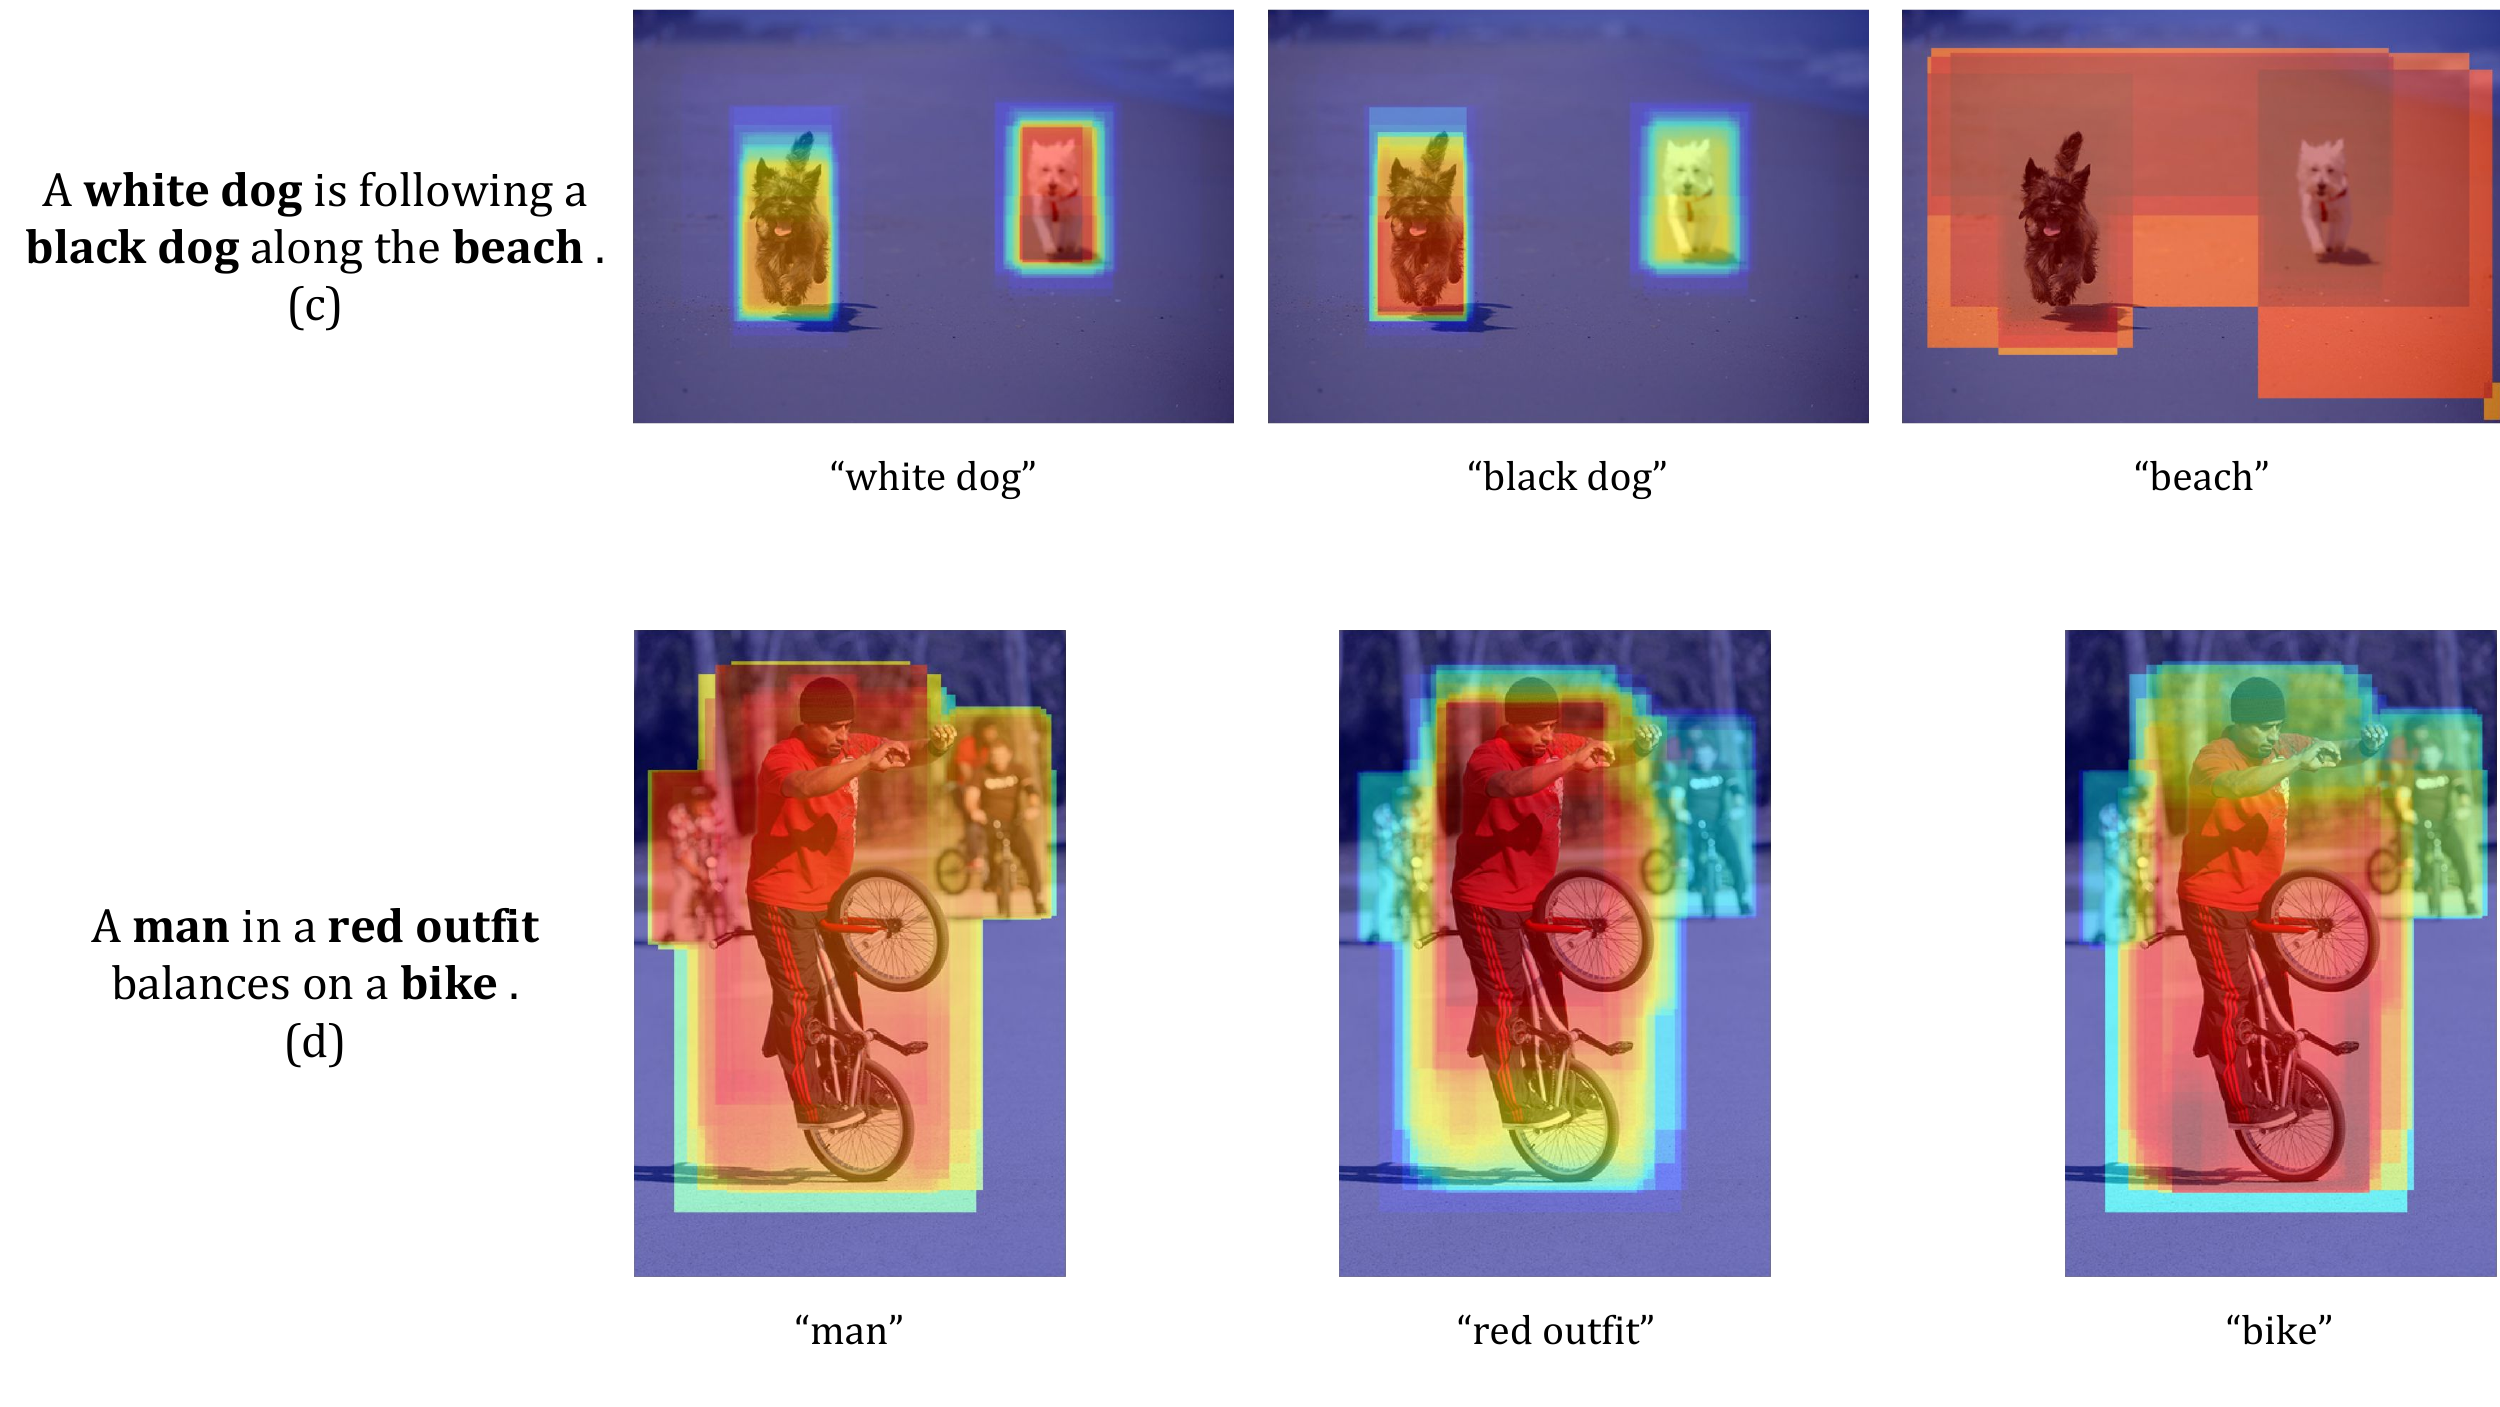}\vspace{-1em}
  \caption{Visualization of region-phrase matching results using our full model (NCE+Distill) on Flickr30k Entities dataset. We present 4 sample images (a—d). For each sample, from left to right: the sentence with parsed phrases, the attention map of region-phrase matching for each phrase. For each pixel, we compute a matching score by averaging scores from all proposals covering the pixel. The red color corresponds to high matching scores.}
\label{fig:grounding-flickr}
\end{figure*}

\begin{figure*}[t]
\centering
\includegraphics[width=1.0\textwidth]{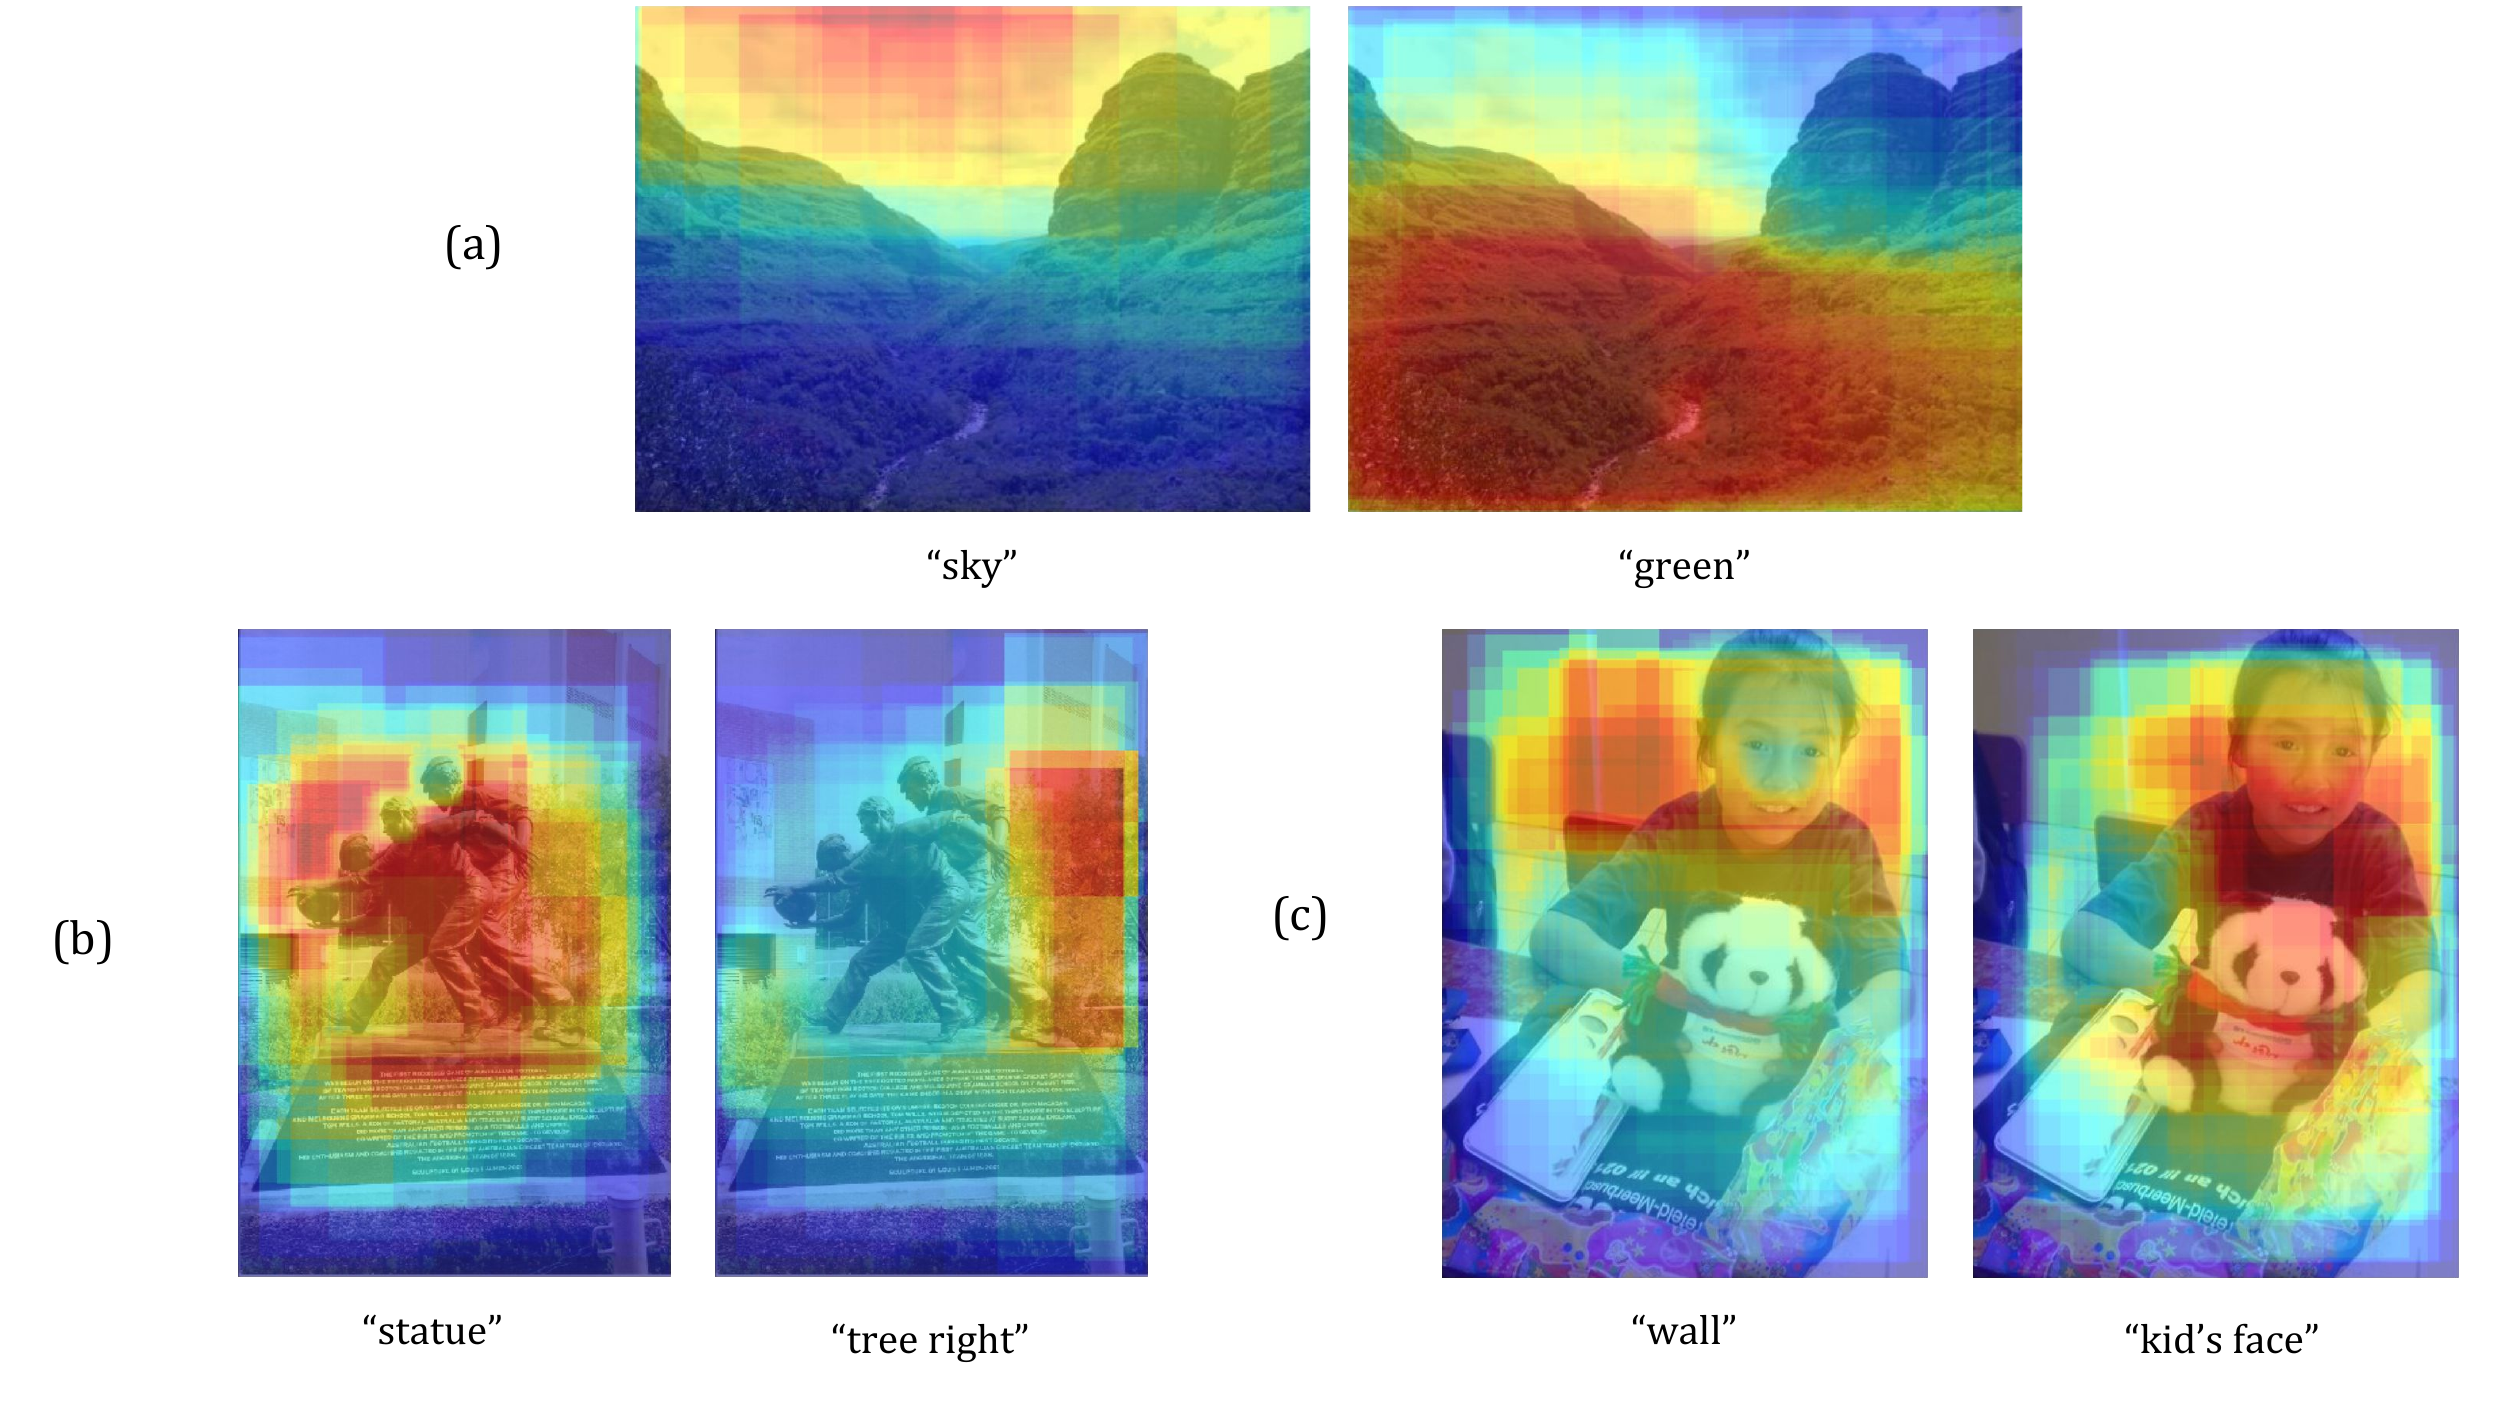}
\includegraphics[width=1.0\textwidth]{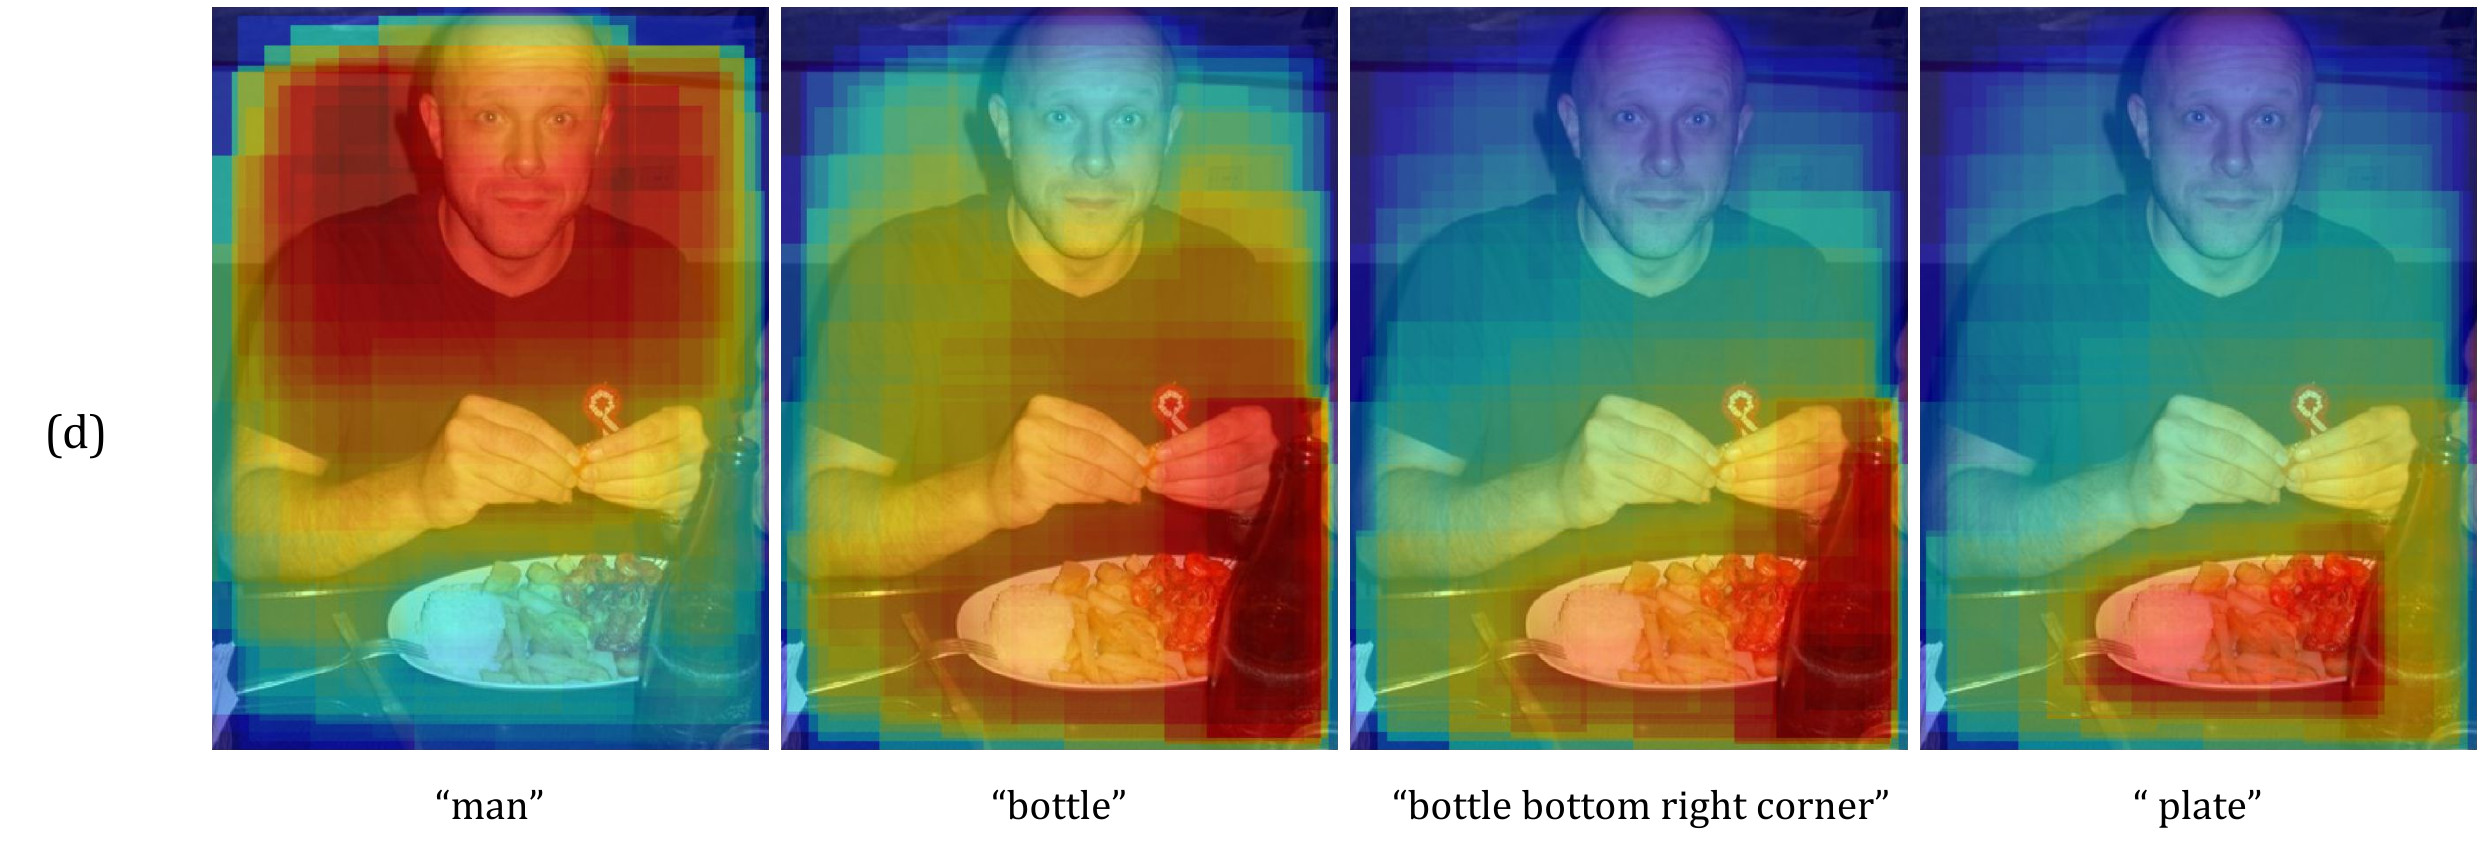}\vspace{-0.6em}
  \caption{Visualization of region-phrase matching results using our full model (NCE+Distill) on ReferItGame dataset. We present 4 sample images (a---d). For each sample, we visualize the attention map of region-phrase matching for each phrase. Similarly, we aggregate matching scores for each pixel from all nearby proposals. The red color corresponds to high matching scores.}
\label{fig:grounding-referit}
\end{figure*}
